# Supplementary material for: Attospiral generation upon interaction of circularly polarized intense laser pulses with cone-like targets
Source: arXiv:1509.06539 ancillary file (2015-09-22)
Supplement: Supplementary file 1 [file suplementf.pdf]

# Supplementary material for the manuscript

Z. Lecz, A. Andreev

(Dated: September 22, 2015)

## I. SPATIAL DISTRIBUTION OF ELECTRONS AND RADIATION

The results presented here support the three dimensional simulations discussed in the manuscript. The situation illustrated in Fig. 1 corresponds to a circularly polarized (CP) laser pulse interacting with a flat foil such that the laser pulse is incident upon the edge of the overdense plasma. By changing the propagation angle of the pulse, with respect to the $x$ direction ($\alpha$), the transition from a cylinder ($\alpha = 0$) to a cone target ($\alpha > 0$) can be reproduced in 2D geometry. The interaction and longitudinal electron motion is identical in 3D space but an additional degree of freedom appears in the azimuthal direction, which will influence the emission angle of the attopulses. The spatial distribution of the high frequency radiation can be obtained by spectral filtering of the electromagnetic waves in the $k$ space, similarly to the one presented in Ref. [1].

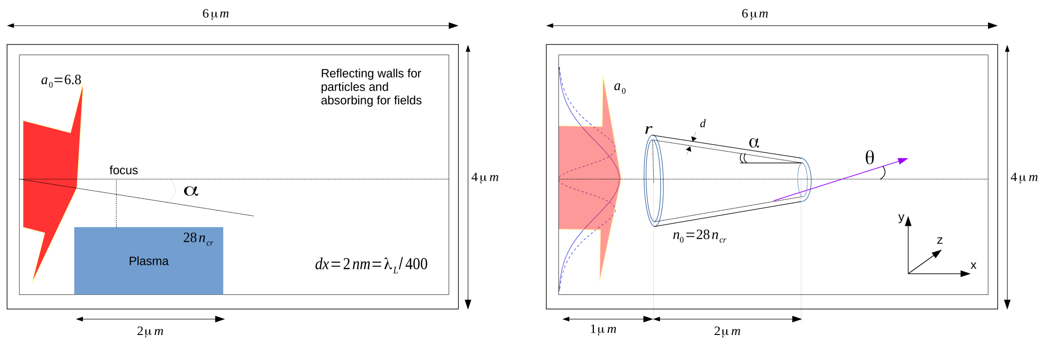


FIG. 1. Sketch of the 2D (left) and 3D (right) simulation domain and parameters.

The Fourier transform of the EM fields is calculated in the spatial domain then the attopulses are reconstructed using the fields propagating with wave numbers larger than 5 times the main wave number ($k > 5k_L$). The maximum harmonic number associated with the plasma oscillations is $\sqrt{28} \approx 5$, thus frequencies above this value are used in order to include attopulses originated from the electron bunches. A basic FFT routine yields the complex numbers $F_k = F_r + iF_i$, where $F_r$ is the real part and $F_i$ is the imaginary part of the field components $F_k$ ($F$ can be electric, $E$, or magnetic, $B$, field). Finally for the representation of the attopulses we used the following formula:

$$F(x) = \sum_k F_r \cos(kx + \varphi_k), \tag{1}$$

where $\varphi_k = arctan(F_i/F_r)$ is the phase corresponding to the given harmonic number. Here $k$ and $x$ are discrete arrays and their length (number of elements) depends on the simulation domain and resolution. In this study, the FFT sampling is made using 2000 grid points, which means $x = 4\,\mu$m longitudinal length. This technique can be also be applied analogously in the time domain.

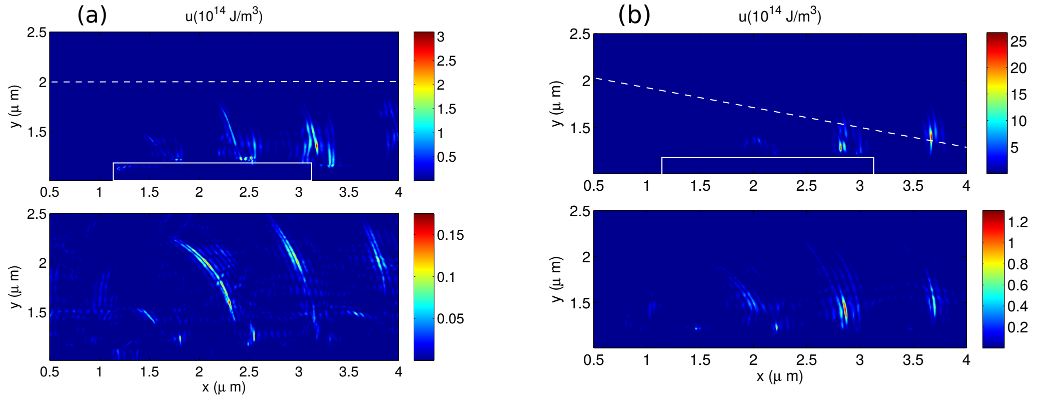


FIG. 2. Energy density of higher harmonics for $\alpha = 0$ (a) and $\alpha = 12$ degrees (b) incidence angle at $t = 18$ fs. The laser pulse enters the simulation at $y = 2\,\mu$m and 2.2 $\mu$m, respectively. Wavelengths shorter than 5 times the laser wavelength are included. The upper and lower panels show the $y$ and $z$ components of the E-field.

The energy density in the reflected attopulses can be seen in Fig. 2a for tangential incidence and for large incidence angle in Fig. 2b. The pulse field amplitude is 3 times larger for oblique incidence and in both cases, attopulses containing the $y$ component are much stronger. The $y$ and $z$ components of the laser field can generate attopulses with very similar emission angles in Fig. 2b, but they propagate in different directions in the left picture. For $\alpha = 0$ the component perpendicular to the plasma surface ($y$) generates attopulses that propagates closer to the plasma, while the tangential component (perpendicular to the plane of simulation) is responsible for the attopulse emitted at the slightly larger angle. The large emission angle will result in radially propagating attopulses in 3D, which get focused right behind the cylinder target in a larger focal spot. In the case of cone target, the atto-spiral will be more confined, because of the narrower and more collinear attopulse emission (see Fig. 2b).

Fig. 3a shows that an electron jet appears above the surface in one half period of the

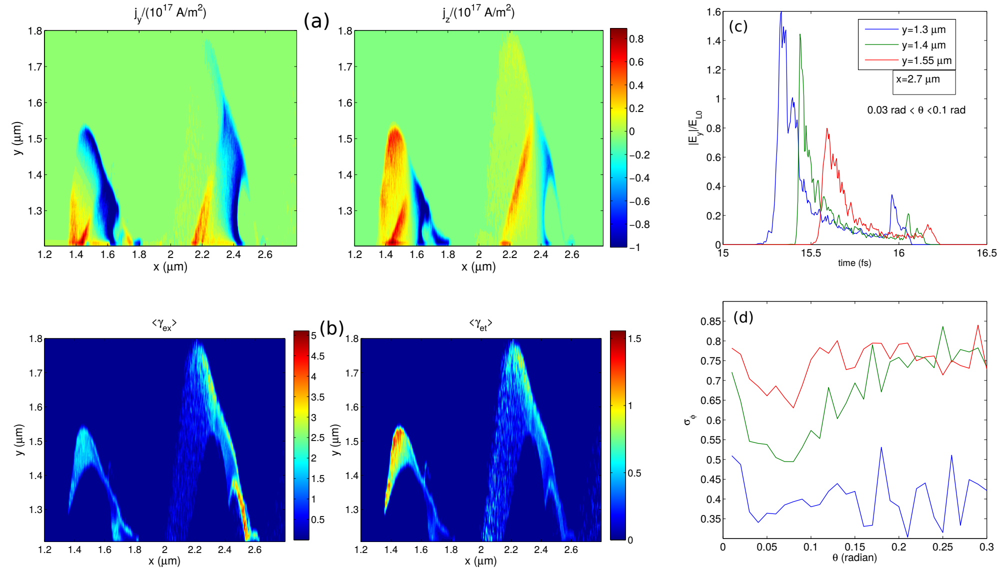


FIG. 3. Transversal current distributions at 11.9 fs for tangential incidence (a). The corresponding electron $\gamma$ distribution (longitudinal - $\gamma_{ex}$ and transversal - $\gamma_{et}$) at the same time instance (b). Only electrons with $\gamma_{ex} > 5$ are included. In (c) the emitted attopulses are shown along three different lines. Below (d) the degree of coherence as a function of emission angle is shown for each line (the color code is the same).

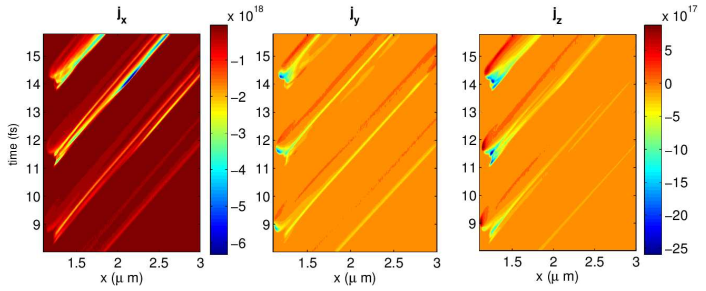


FIG. 4. The $x, y, z$ components of the current density at $y = 1.22$ $\mu$m (0.02 $\mu$m far from the plasma surface). It is measured in the simulation corresponding to Fig. 5. The color is shown in linear scale.

laser (when the electric field, $E_y$, is negative). At the front of this broad peak, the electrons are quickly accelerated and compressed by the ponderomotive force and travel together with the pulse with nearly the speed of light (Fig. 3(b)). They experience a nearly-constant ponderomotive potential in the moving frame of the laser pulse. Although the transversal current density is low, the electron bunch travels almost parallel with the surface (in the

$x$ direction) and the amplitude of emitted field can be higher than the driving laser field. The transversal velocity in the electron bunch crosses the zero point (changes sign) thus the acceleration is highest here for the maximum value of $\gamma_{ex}$ .

These conditions are ideal for efficient attopulse generation via synchrotron emission [2]. The pulse is coherent because of the short duration of the electron bunch. The thin layer of relativistic electrons can be seen in Fig. 3(b) near the plasma edge, where the value of $\gamma_{ex}$ is maximum. Pictures (c) and (d) confirm that the more coherent nature of the radiation and increased intensity of the attopulse is related to the electron nano-bunches, which are formed close to the plasma surface. The degree of coherence is calculated in the same way as in the main text, except that only the $E_y$ component is considered. The $z$ component of the current density changes its sign, farther from the surface, at $y \approx 1.6\mu$m. Thus, the s-polarized attopulses are emitted farther from the plasma surface, also observable in Fig. 2a. The lower energy density of these pulse is explained by the lower electron density at this distance from the target.

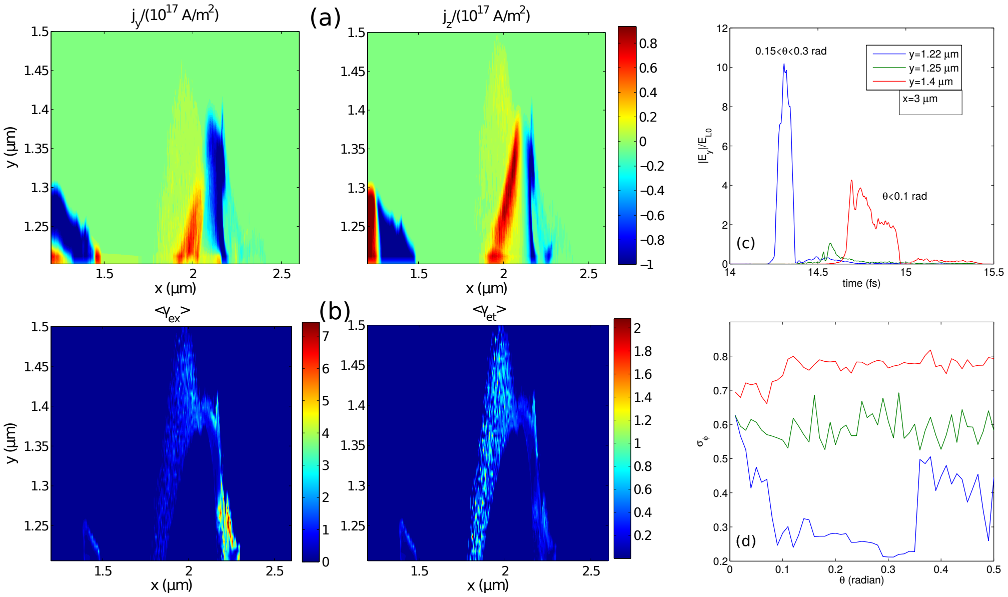


FIG. 5. Transversal current distributions at 11.9 fs for oblique incidence (a). The corresponding electron $\gamma$ distribution (longitudinal - $\gamma_{ex}$ and transversal - $\gamma_{et}$) at the same time instance (b). Only electrons with $\gamma_{ex} > 5$ are included. In the right the same quantities are shown as in Fig. 3c and d.

Fig. 4 shows the current density components in the $(x, t)$ plane and also shows that

the bunch trajectory can be described by linear motion: $x \approx ct$. The incidence is oblique ($\alpha = 0.2$ rad) and the corresponding electron distribution and attopulse emission is shown in Fig. 5. Each straight continuous trace given by the electron bunch in Fig. 4 corresponds to a well defined attopulse. The blue line in Fig. 5c is the result of the straight yellow line starting from $t = 8.5$ fs in the middle panel of Fig. 4 ($j_y$). The attopulse intensity is much higher than in the previous case because the higher intensity part of the laser pulse also interacts with the plasma and the radiation is more coherent. The separation between these sources of coherent radiation along the $x$ axis is exactly $\lambda/4 = 0.2\,\mu$m in the previous case, while in the case of oblique incidence (Fig. 5(a,b)) they almost coincide resulting in a vertical shape of the electron layer. The $y$ and $z$ components of attopulses are emitted by the same electron bunch which explains the identical propagation angles observed in Fig. 2b.

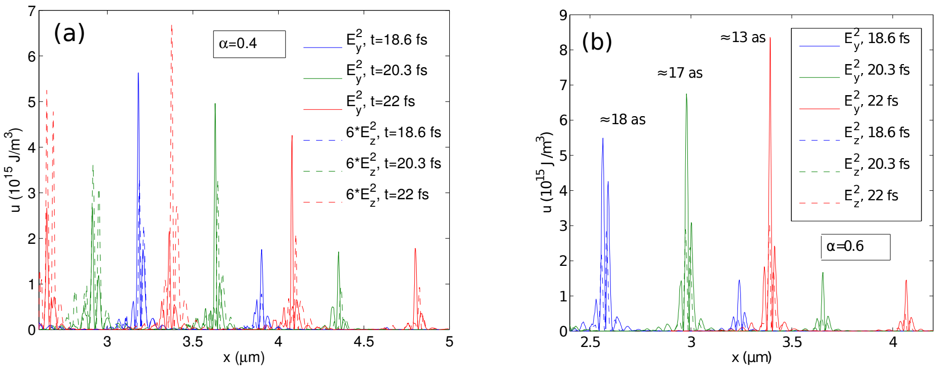


FIG. 6. Energy density of attopulses along the reflection direction at different time instances during vacuum propagation. The time values near the peaks show the full width half maximum values of the pulse duration.

The characteristics of radiation emission observed are also valid in 3D where focusing plays an important role due to the cylindrical geometry. In the case of cylinder target, the tangential component of the laser electric field will be partly transformed into attopulses propagating toward a center, where they are focused near the target rear side. A cone target corresponds to the oblique incidence presented here, when all of the high frequency radiation propagates very close to the plasma surface and the direction is defined by the inner surface of the cone.

During vacuum propagation, the intensity and duration of the attopulses changes due to diffraction effects and/or divergence. In Fig. 6a the attopulse energy density is measured

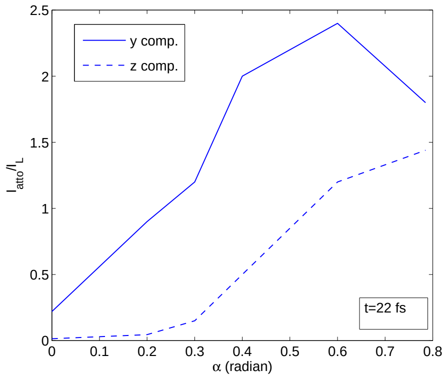


FIG. 7. Maximum peak intensity of the strongest attopulse versus incidence angle. In all cases $I_L = 10^{20}$ W/cm$^2$.

along the axis of propagation. It can be seen that the peak intensity of the $y$ component decreases in time, while $z$ component (dashed line) of the third bunch increases, which can be attributed to the coherent focusing (CHF) [3]. Further simulations show that this effect is more significant at larger $\alpha$ angles (Fig. 6b), which suggests that in the laser spot area the ponderomotive pressure modifies the surface such that the high frequency harmonics constructively overlap for larger distances. The duration of attopulses is of the order of 10 as, which is 10 times smaller than the 3D case (main text), because of the higher $\gamma$ value and the inclusion of frequencies greater than $5\omega_L$ in the spatial filtering. In the main text, the temporal shape is presented which also includes the divergent part and lower frequencies. In the case of $\alpha = 0.6$, the attopulse intensity strongly increases during vacuum propagation, which deserves more attention in future studies.

In Fig. 7 it can be seen that the intensity up-conversion almost reaches $2.5E_{L0}$ but this can change due to vacuum propagation and thus depends on time. As the $\alpha$ angle increases, the attopulse intensity decreases and goes to zero at 90 degrees, because at normal incidence, the CP pulse can not generate high harmonics. The optimal incidence angle is between 30-40 degrees, where the center of the laser pulse also interacts with the plasma. This is is not feasible in 3D space with cone-like targets and for the realization of such interaction, a curved plasma surface with curvature radius similar to the laser focal spot radius would be required.

## II. HARMONIC SPECTRUM

Attopulses are produced by relativistic electrons near the plasma surface, the location of the maximum ponderomotive force and the vector potential ($\mathbf{A}_\perp$, the component perpendicular to the plasma surface) varies slowly in the moving frame of the electron bunch. In this frame, we can introduce the simplest time dependence around zero: $A_\perp(t \approx 0) = A_0(1-t^n)$, which appears in the equation of motion: $\partial\mathbf{p}/\partial t = -m_e c^2 \nabla(\sqrt{1+e^2A_\perp^2(t)/m_e^2c^2} - 1)$, where the space charge field outside of the plasma is neglected. By substituting $p \approx p_x = m_e v_x/\sqrt{1-v_x^2/c^2}$ and replacing the spatial derivative with $1/dx = 1/cdt$ one arrives to the expression:

$$v_x/c = \sqrt{\frac{2+\tau^2+\tau^4-2\sqrt{1+\tau^2}}{5+2\tau^2+\tau^4}}, \tag{2}$$

where $\tau = a_0(1-t^n)$ and $a_0 = eA_0/(m_e c)$. For the calculation of the spectral intensity it is necessary to obtain the time dependent trajectory of the electrons, $x(t)$. It is impossible to integrate $v_x$ given in Eq. (5), but this expression can be fitted to a polynomial function of the form $v_x(t) = v_0(1-\alpha_1 t^{2n})$, where $v_0$ is the maximum velocity achieved during the running time, and we found that $\alpha_1 \approx 6/a_0^3$. This time dependence is used for the longitudinal velocity instead of Eq. (1) from [2]. The calculation is performed in the moving frame, thus retarded time is used: $ct' = ct + x(t') - x$. Starting from the general expression of Lienard-Wiechert potentials, the electric field can be expressed as [2]:

$$E(t') \propto \frac{a_y(t')}{(1-v_x(t')/c)^2}, \tag{3}$$

where the transversal acceleration ($a_y$) is approximated with a Gaussian function. After the integration of $v_x(t')$ and inserting $x(t')$ into the expression of retarded time the following relation is obtained:

$$t' = \frac{(t-x/c)2\gamma^2}{1+2\alpha_1\gamma^2 t'^{2n}/(2n+1)}. \tag{4}$$

For $n = 1$, the solution of the above expression can be approximated with an interpolation function, given in [2]. In this case, it is numerically solved by using the replacement $t - x/c = t \ll 1$ and the discrete data to obtain the electric field in time. The graphical representation is shown in Fig. 8a for $n = 7$, $\gamma = 3$ and $a_0 = 5$. It can be seen that $v_x$ is nearly constant

in the vicinity of the moment of pulse emission and $t'(t)$ undergoes a rapid growth in this time interval.

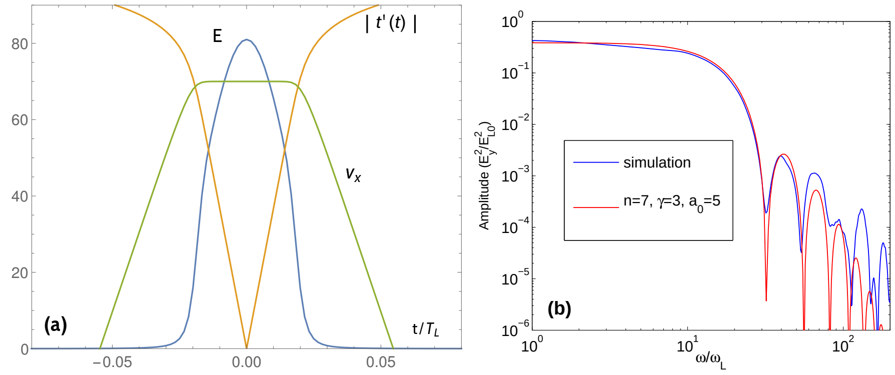


FIG. 8. The modulus of retarded time (yellow), longitudinal velocity (green) and electric field (blue) is shown versus time (a). In (b) the discrete Fourier transform (red) of the electric field is compared to the spectrum of the attopulse presented in Fig. 5c with blue line.

In Fig. 8b the discrete Fourier transform (absolute value) of the $E$ field (blue line) is in a very good agreement (except the high frequencies) with the simulation result. The blue line spectrum is the Fourier transform of the attopulse shown in Fig. 5c with the same color. The fitting parameters $n, \gamma$ can be accurately obtained because the value of $n$ is responsible for the number of bumps present in the spectrum and also defines the steepness of the spectrum. The value of $\gamma$ is mainly related to the high frequency cut-off and defines the position of the first modulation along the frequency coordinate. In the main text, we have chosen the CSE spectrum expressed by Airy functions. Here we see that this spectrum (obtained numerically from Eq. 3) better describes the spectrum of emitted radiation because it is constant in the low frequency region. We can not also provide an analytical expression for it. The difference between the two models lays in the approximation of the transversal acceleration (or velocity). The Gaussian function seems to be more accurate but it results in making the analytical derivation of the spectral intensity more complex and difficult.

We observe that in the case of grazing incidence (which is more possible in experiments) higher values of $n$ and $\gamma$ are used for fitting, because the higher intensity parts of the laser pulse also interacts with the plasma, allowing electrons to gain more energy. The electron bunch is also more compressed and is accelerated more quickly resulting in a longitudinal velocity very close to speed of light during almost the whole path of motion. Mathematically,

it means that the function $v(1-t^{2n})$ tends to a constant value (approaches $v_{max} \approx c$) as the value of $n$ is increased.

---


[1] C. Hernández-García et al., Phys Rev Lett **111**, 083602 (2013)

[2] J. M. Mikhailova et al., Phys Rev Lett **109**, 245005 (2012)

[3] S. Gordienko et al., Phys Rev Lett **94**, 103903 (2005)
